# Supplementary material for: On-Chip Microwave Quantum Hall Circulator
Source: arXiv:1601.00634 source file (2016-01-04)
Supplement: Supplementary file 1 [file supplemental_SUBMIT.pdf]

Science
AAAS

# Supplementary Materials for
# On-Chip Microwave Quantum Hall Circulator

A. C. Mahoney* [1,2], J. I. Colless* [1,2], S. J. Pauka[1,2], J. M. Hornibrook[1,2], J. D. Watson [3,4], G. C. Gardner[4,5], M. J. Manfra[3,4,5], A. C. Doherty[1], and D. J. Reilly† [1,2]

[1] ARC Centre of Excellence for Engineered Quantum Systems, School of Physics, The University of Sydney, Sydney, New South Wales 2006, Australia.

[2] Microsoft Station Q Sydney, The University of Sydney, Sydney, New South Wales 2006, Australia.

[3] Department of Physics and Astronomy, Purdue University, West Lafayette, Indiana 47907, USA.

[4] Birck Nanotechnology Center, School of Materials Engineering and School of Electrical and Computer Engineering, Purdue University, West Lafayette, Indiana 47907, USA.

[5] Microsoft Station Q Purdue, Purdue University, West Lafayette, Indiana 47907, USA.

∗These authors contributed equally to this work.
†To whom correspondence should be addressed; E-mail: david.reilly@sydney.edu.au

**This PDF file includes:**

Materials and Methods
Supplementary Text
Fig. S1
Fig. S2

# I. MATERIALS AND METHODS

## A. Devices:

All devices are fabricated on GaAs/AlGaAs heterostructure with a 2-dimensional electron gas (2DEG) located 270 nm below the surface. From dc Hall transport measurements, an electron density of $n_s = 1.1 \times 10^{11}$ cm$^{-2}$ is extracted, along with carrier mobility of $\mu = 5.2 \times 10^6$ cm$^2$/Vs. Circular mesa disks are etched using a $H_2 0/H_2 0_2/H_2SO_4$ solution to a depth of $\sim$ 320 nm.

Metallic Ti/Au is evaporated on top of the devices to form the waveguide and circulator port structures. For the transmission-line device shown in Fig. 1 of the paper, a coplanar transmission line geometry is employed using a 50 µm wide signal track with ground planes on either side. The distance to these ground planes measures 30 µm, ensuring a coupling impedance of $\sim$ 50 Ω within the frequency range of operation. The 350 µm diameter disc is situated equidistant between the signal line and ground plane, with a gap of 20 µm at either side. For the three-port device, a 330 µm diameter disk is placed at the center of the structure, with metallic ports separated by 20 µm from the mesa. The edges of the ports form 250 µm long curved arcs, and a surrounding ground plane is separated back from the disc by 385 µm.

The data in Fig. 1C is taken on a device with an additional 100 µm diameter ohmic contact placed in the center of the mesa to assist in thermalization of the isolated disk of electron gas. This contact does not intersect the edge and as such we find that the absorption spectrum (Fig. 1C) is qualitatively the same for devices without a center ohmic contact.

## B. Circuit setup:

All measurements are performed at the base temperature T $\sim$ 20 mK of a cryo-free dilution refrigerator (Leiden Cryogenics CF650). Semi-rigid coaxial cables are attenuated by 12 dB from the top to the bottom of the fridge for improved thermalization, while the return line $2'$ is amplified at the 4 K stage of the fridge with a low-noise, resistive-feedback, cryogenic amplifer (Weinreb group, Caltech) with a noise temperature of $\sim$ 5 K and Gain = 40 dB. The return signals are further amplified at room temperature. For the data shown in the paper, the applied microwave power at the device was in the range -90 dBm to -60 dBm. Features appear sharper at lower microwave power, but with a decrease in signal to noise.

Devices are mounted on two layer copper printed circuit boards (PCBs) constructed from Rogers 6006 high frequency laminate. These are mounted flat on a copper stage, which is thermally anchored to the mixing chamber plate of the dilution refrigerator (Fig. S1). A cut-out in the PCBs enables devices to be silver pasted directly onto the copper beneath, ensuring good thermal contact. The ground planes of the devices are electrically connected to the ground of the PCB using numerous aluminum bondwires.

Chip-inductors (47 nH) are copper-wound, Coilcraft (0805HT series) and bonded to each of the three ports of the circulator to form an impedance matching network. The inductors are found to resonate with the stray parasitic capacitance in the setup $C_{\mathrm{stray}}$, at a frequency of $\sim$ 1 GHz in the absence of a magnetic field.

## C. Experimental methods:

$S$-parameter measurements are taken with a Keysight N5245A PNA-X network analyzer. For the setup in Fig. 4 E and F, an E8267D vector signal generator is used to output a 1 GHz continuous wave which is then modulated with a Gaussian envelope via an AWG 5014C arbitrary waveform generator before being directed to port-1 of the device. A mechanical switch (Radiall DPDT series) mounted on the mixing chamber stage of the fridge enables the output lines 2 and 3 to be selectively directed through a common return line that is amplified by the cryogenic amplifier. The resultant signal is measured with a digital sampling oscilloscope and and a fast Fourier transform (FFT) is performed in post-processing.

## II. SUPPLEMENTARY TEXT

### A. Extracting the dielectric permittivity:

The overall dispersion curve of the fundamental edge magnetoplasmon (EMP) mode is extracted from the position of the features in the 2D data, as shown in the inset of Fig. 1C. Black markers plot the center frequency for which the features occur, measured at magnetic field values corresponding to integer filling factors $\nu$, down to $\nu = 2$, (errors are within the square marker bounds). The black solid line shows a fit to the resulting 1D data using the nonlinear dispersion relation for the fundamental mode $\omega = \frac{\sigma_{\mathrm{edge}} q}{2\pi\varepsilon^* \varepsilon_0}\left[\ln\frac{2}{ql} + c\right]$ (see Refs. [18-25] in the main paper for derivation of this expression). Here $\omega = 2\pi f$, $\sigma_{\mathrm{edge}}$ is the transverse conductivity of the edge, $\varepsilon^*$ and $\varepsilon_0$ are the dielectric constant and permittivity of free space respectively, $c = 1$ for a sharp (etched) edge, and $q = \frac{2\pi}{p}$, where $p$ is the sample perimeter. The parameter $l$ gives the physical extent of the EMP away from the etched edge of the mesa and is approximated by $l = \frac{n_s m^*}{2\varepsilon^* \varepsilon_0 B^2}$ where $n_s = 1.1 \times 10^{11}$ cm$^{-2}$ is the carrier density, and $m^*$ is the effective electron mass in GaAs of 0.067 $m_e$. We extract the free parameter $\varepsilon^* \sim 8.7$ from the fit, consistent with Ref. [25]. This value of $\varepsilon^*$ corresponds to an average of the dielectric constant of GaAs and the vacuum, since the capacitive response of the system includes the edge-state, etched trench, and metallic structure that defines the microwave port.

### B. Theoretical model:

We begin with the admittance matrix $Y_{\mathrm{edge}}$ for a three-port quantum Hall circulator using a Carlin type device, exactly as described in Ref. [9]:

$$Y_{\mathrm{edge}}(\omega) = \begin{pmatrix} ia & b & -b^* \\ -b^* & ia & b \\ b & -b^* & ia \end{pmatrix}$$

Where, as in Ref. [9],

$$a = \frac{2\sigma_{\mathrm{edge}} \sin\frac{\omega C_{\mathrm{edge}}}{\sigma_{\mathrm{edge}}}}{1 + 2\cos\frac{\omega C_{\mathrm{edge}}}{\sigma_{\mathrm{edge}}}}$$

$$b = \sigma_{\mathrm{edge}} \frac{-1 + e^{\frac{-i\omega C_{\mathrm{edge}}}{\sigma_{\mathrm{edge}}}}}{1 + 2\cos\frac{\omega C_{\mathrm{edge}}}{\sigma_{\mathrm{edge}}}}$$

with $\omega$ the angular frequency, $\sigma_{\mathrm{edge}}$ is the conductance of the edge ($1/\sigma_{\mathrm{edge}} = R_{xy}$) and $C_{\mathrm{edge}}$ the contact capacitance between each of the port terminals and the edge. Note this 3 x 3 matrix is not symmetric and thus captures the non-reciprocal response of the chiral edge magnetoplasmons.

We now modify the circuit with respect to Ref. [9], by adding terms to account for dissipation $R$, either along the quantum Hall edge or elsewhere in the circuit, as well as a direct parasitic capacitive path $C_{\mathrm{p}}$, between port terminals. We derive an admittance matrix $Y_{\mathrm{total}}$ which captures these additional terms as a function of $Y_{\mathrm{edge}}$, $R$, and $C_{\mathrm{p}}$.

Referring to the circuit diagram shown in Fig. S2, and given Ohm's law we write:

$$\vec{I'} = Y_{\mathrm{edge}} \vec{V'} \text{ and } \vec{V} = \vec{V'} + R\vec{I'},$$

where $\vec{I'}$ ($\vec{V'}$) are the vectors of currents (voltages) of $Y_{\mathrm{edge}}$ and $\vec{I}$ ($\vec{V}$) are the vectors of currents (voltages) of $Y_{\mathrm{total}}$. Rearranging and substituting we find,

$$\vec{I'} = Y_{\mathrm{res}} \vec{V}, \text{ where } Y_{\mathrm{res}} = (\mathrm{I} + RY_{\mathrm{edge}})^{-1} Y_{\mathrm{edge}} \vec{V} \text{ and I is the identity matrix.}$$

We can then write out the individual components of $\vec{I}$ by summing the net flows in and out of each port of the circulator, as shown in Fig. S2:

$$
\begin{aligned}
I_1 = I'_1 + (I_{12} - I_{31}) = (Y^{11}_{\text{res}} V_1 + Y^{12}_{\text{res}} V_2 + Y^{13}_{\text{res}} V_3) + i\omega C_{\text{p}} (2V_1 - V_2 - V_3) \\
I_2 = I'_2 + (I_{23} - I_{12}) = (Y^{21}_{\text{res}} V_1 + Y^{22}_{\text{res}} V_2 + Y^{23}_{\text{res}} V_3) + i\omega C_{\text{p}} (2V_2 - V_3 - V_1) \\
I_3 = I'_3 + (I_{31} - I_{23}) = (Y^{31}_{\text{res}} V_1 + Y^{32}_{\text{res}} V_2 + Y^{33}_{\text{res}} V_3) + i\omega C_{\text{p}} (2V_3 - V_1 - V_2)
\end{aligned}
$$

and thus,

$$
\vec{I} = Y_{\text{res}} \vec{V} + \begin{pmatrix} 2i\omega C_{\text{p}} & -i\omega C_{\text{p}} & -i\omega C_{\text{p}} \\ -i\omega C_{\text{p}} & 2i\omega C_{\text{p}} & -i\omega C_{\text{p}} \\ -i\omega C_{\text{p}} & -i\omega C_{\text{p}} & 2i\omega C_{\text{p}} \end{pmatrix} \vec{V},
$$

such that we can write:

$$
\vec{I} = Y_{\text{total}} \vec{V}, \text{ where } Y_{\text{total}} = (\mathrm{I} + R Y_{\text{edge}})^{-1} Y_{\text{edge}} + \begin{pmatrix} 2i\omega C_{\text{p}} & -i\omega C_{\text{p}} & -i\omega C_{\text{p}} \\ -i\omega C_{\text{p}} & 2i\omega C_{\text{p}} & -i\omega C_{\text{p}} \\ -i\omega C_{\text{p}} & -i\omega C_{\text{p}} & 2i\omega C_{\text{p}} \end{pmatrix}
$$

Finally we calculate the scattering parameters of the system as a function of the angular frequency $\omega$ via the transformation:

$$
S(\omega) = \left(Z^{-1} + Y_{\text{total}}\right)^{-1} \left(Z^{-1} - Y_{\text{total}}\right) \text{ where } Z = Z_0 \mathrm{I}.
$$

This expression is used to calculate $S_{31}$ and $S_{13}$ and their difference as shown in Fig. 4 of the paper. To compare our model to experimental data in Fig. 4C and 4D, where the background response at zero magnetic field has been subtracted, we normalize the results of the model by setting to $S = 0$ dB the response of just the parasitic path $C_{\text{p}}$. Thus a value of S = 0 dB in Fig. 4 C and D represents the response of the system when no quantum Hall edge is present, similar to the experimental situation at zero field.

To qualitatively compare our model to the experimental data, we account for the 5 variables: the characteristic impedance $Z_0$, the parasitic capacitance $C_{\text{p}}$, the effective capacitance of the quantum Hall edge $C_{\text{edge}}$, the conductance of the edge $\sigma_{\text{edge}} = 1/R_{xy}$, and the total dissipation $R$. To produce qualitative fits to the data, we fix $Z_0$ and vary $R_{xy}$ and $C_{\text{edge}}$ to align the peaks and dips to correspond to the EMP frequencies. Finally, we adjust $C_{\text{p}}$ and $R$ to vary the amplitude and width of the features in our model to fit the corresponding data. Note that the parameters we have chosen fit the data both on and off the EMP resonance by just modifying $R$. Although qualitative, the values of $C_{\text{p}}$ and $R$ chosen in the model are consistent with typical values for the parasitic capacitance and total dissipation estimated via transport measurements and geometric considerations. The caption for Figure 4 in the paper lists the values used in the model.

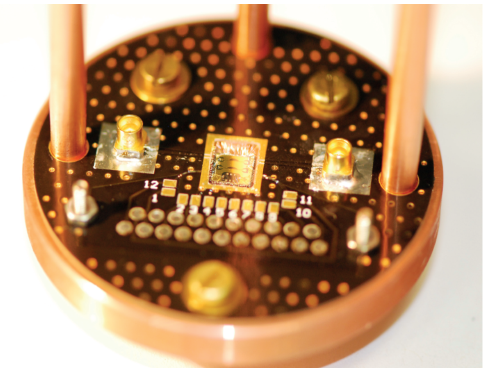

**Fig. S1**
Photograph of a 2-port transmission line device, wire-bonded to the PCB. The PCB is in thermal contact with a copper stage that is mounted to the mixing chamber of a dilution refrigerator.

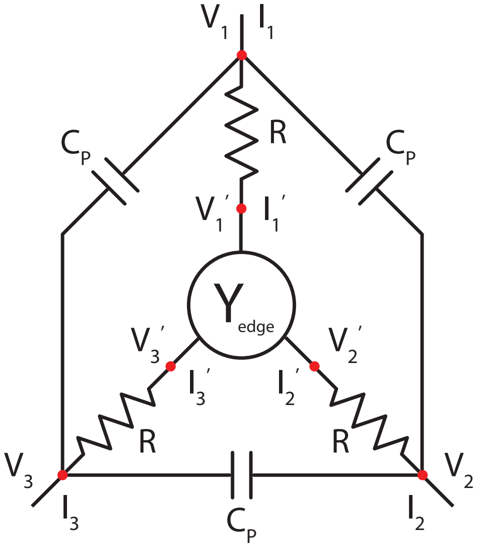


**Fig. S2**
Theoretical circuit model of a three port circulator including dissipation $R$ and direct parasitic capacitive coupling $C_\mathrm{p}$ between port terminals. Nodes where I/I′ and V/V′ are calculated are shown in red.
